# Supplementary material for: A computational model for the evolution of learning physical micro-contents in peer instruction methodology
Source: arXiv:2405.07055 source file (2024-05-11)
Supplement: Supplementary file 1 [file Apen_binomial.tex]

\chapter{Binomial}

A group of $N$ students is taking a test consisting of $n$ multiple-choice questions with only one answer and $s$ answer choices per question. The students are divided into two subgroups, where the $N_1$ students have a probability of $p_1$ to answer correctly each question, and the remaining $N-N_1$ students have a probability of $p_2$ to answer each question. Each student's response is modeled as a binomial distribution with $n$ trials and success probabilities $p_1$ and $p_2$, respectively. Do all $N$ students follow a single global binomial distribution in their answers?

Let $P_1$ and $P_2$ be the binomial distribution of each type of student and $P$ the global binomial distribution, which are given by
%------------
\begin{equation} \label{bino1}  %-
    P_1(k) = \binom{n}{k} p_1^k (1-p_1)^{n-k},
\end{equation}
%-----
\begin{equation} \label{bino2}  %-
    P_2(k) = \binom{n}{k} p_2^k (1-p_2)^{n-k}
\end{equation}
%----
and
\begin{equation} \label{binog}  %-
    P(k) = \binom{n}{k} p^k (1-p)^{n-k}
\end{equation}
%----

Based on the distribution's definition, we know that the probability of failure in each trial is $q_1=1-p_1$ 
and $q_2=1-p_2$, respectively. Now we put two conditions on the response probabilities:
\begin{equation} \label{ap_cod1}  %-
    p = a p_1+b p_2, 
\end{equation}
with $a$ and $b$ constant, that is, $p$ is a linear combination of $p_1$ and $p_2$. The other condition is:
\begin{equation} \label{ap_cod2}  %-
    a+b=1.
\end{equation}.

Substituting (\ref{ap_cod1}) in \ref{binog}, we find 
\begin{equation} \label{profin}  %-
    P(k) = \binom{n}{k} \left (a p_1+b p_2\right ) ^k (1-a p_1-b p_2)^{n-k}
\end{equation}
and since $\left (1-a p_1-b p_2  \right )=\left (a q_1+ b q_2  \right )$ then we  find
\begin{equation} \label{casfin}  %-
    P(k) = \binom{n}{k} \left (a p_1+b p_2\right ) ^k (a q_1+b q_2)^{n-k}, 
\end{equation}
since $q=a q_1+b q_2$.
\begin{equation} \label{tbino} 
(a q_1 + b q_2)^n = \sum_{k=0}^n \binom{n}{k} \left (a q_1 \right )^{n-k} \left (a q_1 \right )^k  
\end{equation}
